# Supplementary material for: Dynamic Correlation Clustering in Sublinear Update Time
Source: arXiv:2406.09137 source file (2024-06-13)
Supplement: Supplementary file 1 [file Appendix.tex]

\newpage
\appendix
\onecolumn

\input{AgreementAndHeavinessCalculation}
\input{StructuralProperties}
\input{Notify}
\input{DenseClustersFinding}
\input{AllFoundClustersAreDense}
\input{RuntimeAnalysis}
\input{ClusteringComputationFromSparseSolution}
